# Supplementary material for: Optimal query complexity for estimating the trace of a matrix
Source: arXiv:1405.7112 source file (2014-05-28)
Supplement: Supplementary file 1 [file appendix.tex]

% !TEX root =main.tex
